# Supplementary material for: The Maximum $T_c$ of Conventional Superconductors at Ambient Pressure
Source: arXiv:2502.18281 source file (2025-02-25)
Supplement: Supplementary file 1 [file Suppl.pdf]

# Supplementary Information for: The Maximum $T_c$ of Conventional Superconductors at Ambient Pressure

Kun Gao,<sup>1</sup> Tiago F. T. Cerqueira,<sup>2</sup> Antonio Sanna,<sup>3</sup> Yue-Wen Fang,<sup>4</sup> Đorđe Dangić,<sup>4,5</sup>  
Ion Errea,<sup>4,5,6</sup> Hai-Chen Wang,<sup>1</sup> Silvana Botti,<sup>1</sup> and Miguel A. L. Marques<sup>1,\*</sup>

<sup>1</sup>*Research Center Future Energy Materials and Systems of the University Alliance Ruhr and Interdisciplinary Centre for Advanced Materials Simulation, Ruhr University Bochum, Universitätsstraße 150, D-44801 Bochum, Germany*

<sup>2</sup>*CFisUC, Department of Physics, University of Coimbra, Rua Larga, 3004-516 Coimbra, Portugal*

<sup>3</sup>*Max-Planck-Institut für Mikrostrukturphysik, Weinberg 2, D-06120 Halle, Germany*

<sup>4</sup>*Centro de Física de Materiales (CFM-MPC), CSIC-UPV/EHU, Manuel de Lardizabal Pasealekua 5, 20018 Donostia/San Sebastián, Spain*

<sup>5</sup>*Fisika Aplikatua Saila, University of the Basque Country (UPV/EHU), Europa Plaza 1, 20018 Donostia/San Sebastián, Spain*

<sup>6</sup>*Donostia International Physics Center (DIPC), Manuel de Lardizabal Pasealekua 4, 20018 Donostia/San Sebastián, Spain*

(Dated: February 25, 2025)

---

\* miguel.marques@rub.de

#1:  $\text{Tl}_2\text{AgH}_2$ 

mat id agm002924843  
 spg 139  
 nsites 5  
 e above hull 0.124 eV  
 e form 0.101 eV  
 decomposition Tl, Ag,  $\text{TlH}_4$   
 ecutwfc 100.0 Ry  
 kpts coarse  $16 \times 16 \times 16$   
 kpts fine  $32 \times 32 \times 32$   
 qpts  $4 \times 4 \times 4$   
 $\lambda$  1.128  
 $\omega_{\text{log}}$  141 K  
 $\omega_2$  475 K  
 $T_{\text{c}}^{\text{McMillan}}$  11.7 K  
 $T_{\text{c}}^{\text{Allen-Dynes}}$  12.7 K  
 $T_{\text{c}}^{\text{Eliashberg}}$  13.2 K

**Primitive structure:**

$a$ : 5.0017 Å,  $b$ : 5.0017 Å,  $c$ : 5.0017 Å  
 $\alpha$ : 118.36°,  $\beta$ : 118.36°,  $\gamma$ : 92.87°

Tl [0.7500, 0.2500, 0.5000]  
 Tl [0.2500, 0.7500, 0.5000]  
 Ag [0.0000, 0.0000, 0.0000]  
 H [0.5555, 0.5555, 0.0000]  
 H [0.4445, 0.4445, 0.0000]

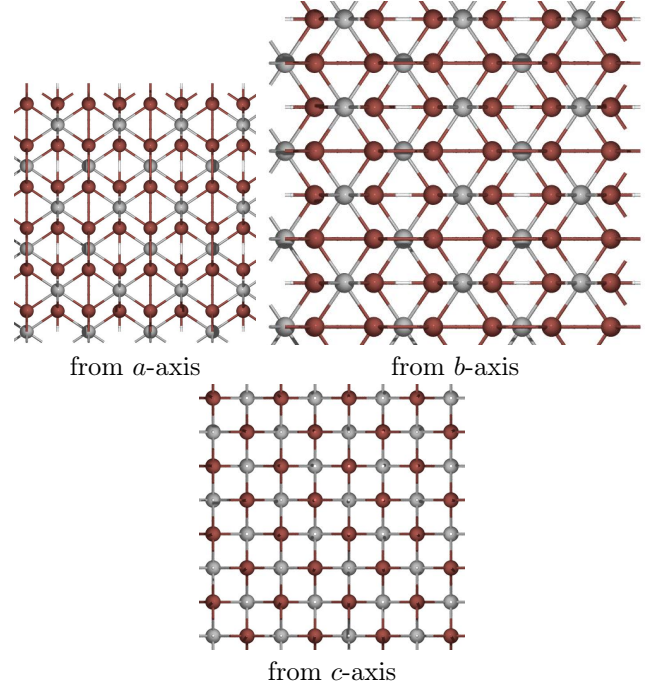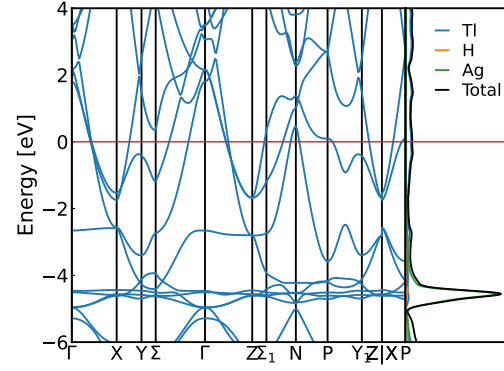

Electron band structure

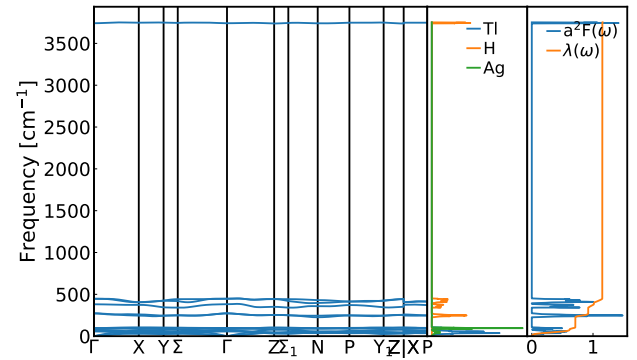

Phonon band structure

#2: NaNiH<sub>3</sub>

mat id agm002490730  
 spg 221  
 nsites 5  
 e above hull 0.014 eV  
 e form -0.241 eV  
 decomposition NaNiH<sub>3</sub>  
 ecutwfc 116.0 Ry  
 kpts coarse 16×16×16  
 kpts fine 32×32×32  
 qpts 4×4×4  
 λ 0.158  
 ω<sub>log</sub> 1090 K  
 ω<sub>2</sub> 1420 K  
 T<sub>c</sub><sup>Mcmillan</sup> 0.0 K  
 T<sub>c</sub><sup>Allen-Dynes</sup> 0.0 K  
 T<sub>c</sub><sup>Eliashberg</sup> 0.0 K

**Primitive structure:**

$a$ : 3.3957 Å,  $b$ : 3.3957 Å,  $c$ : 3.3957 Å  
 $\alpha$ : 90.00°,  $\beta$ : 90.00°,  $\gamma$ : 90.00°

Na [0.5000, 0.5000, 0.5000]  
 Ni [0.0000, 0.0000, 0.0000]  
 H [0.0000, 0.5000, 0.0000]  
 H [0.0000, 0.0000, 0.5000]  
 H [0.5000, 0.0000, 0.0000]

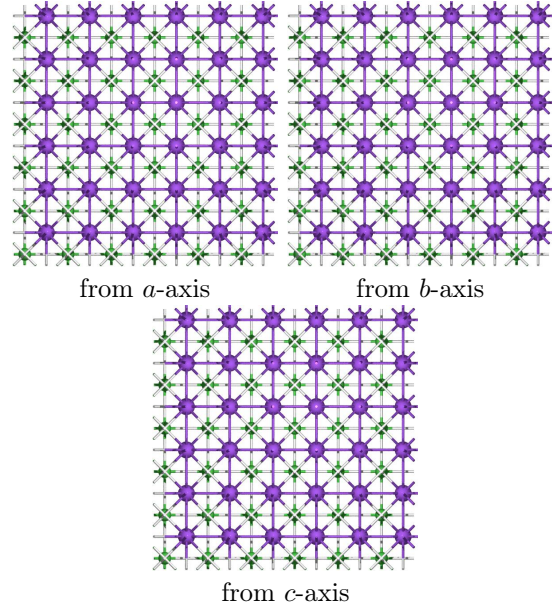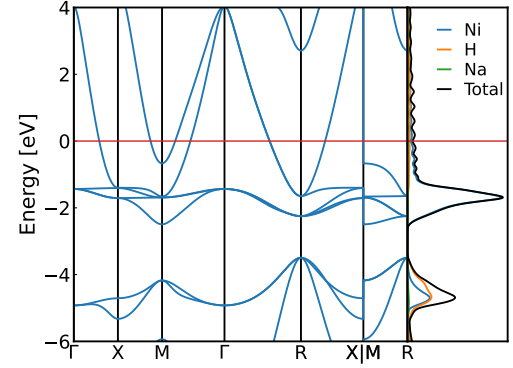

Electron band structure

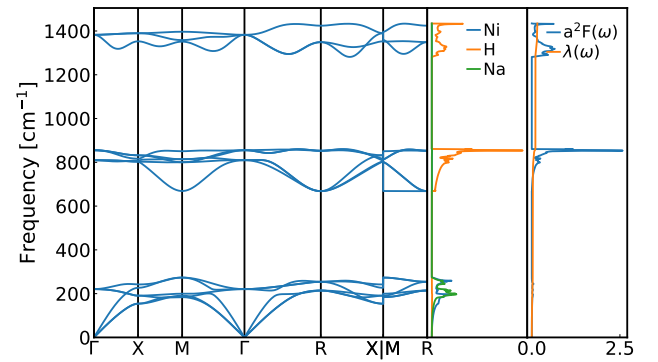

Phonon band structure

#3: BC<sub>11</sub>

```

mat id agm006148322
spg 21
nsites 12
e above hull 0.225 eV
e form 0.214 eV
decomposition C, B4C
ecutwfc 90.0 Ry
kpts coarse 12×12×16
kpts fine 24×24×32
qpts 3×3×4
λ 0.551
ωlog 1193 K
ω2 1269 K
TcMcmillan 20.7 K
TcAllen-Dynes 21.2 K
TcEliashberg 24.0 K

```

**Primitive structure:**

$a$ : 5.7150 Å,  $b$ : 5.7150 Å,  $c$ : 3.5998 Å  
 $\alpha$ : 90.00°,  $\beta$ : 90.00°,  $\gamma$ : 143.32°

```

B [0.0000, 1.0000, 0.5000]
C [0.1696, 0.3409, 0.7555]
C [0.3332, 0.6668, 0.5000]
C [0.5000, 1.0000, 0.7471]
C [0.1673, 0.8327, 0.0000]
C [0.3409, 0.1696, 0.2445]
C [0.6668, 0.3332, 0.5000]
C [0.8304, 0.6591, 0.7555]
C [0.5000, 0.5000, 0.0000]
C [0.6591, 0.8304, 0.2445]
C [0.8327, 0.1673, 0.0000]
C [0.0000, 0.5000, 0.2529]

```

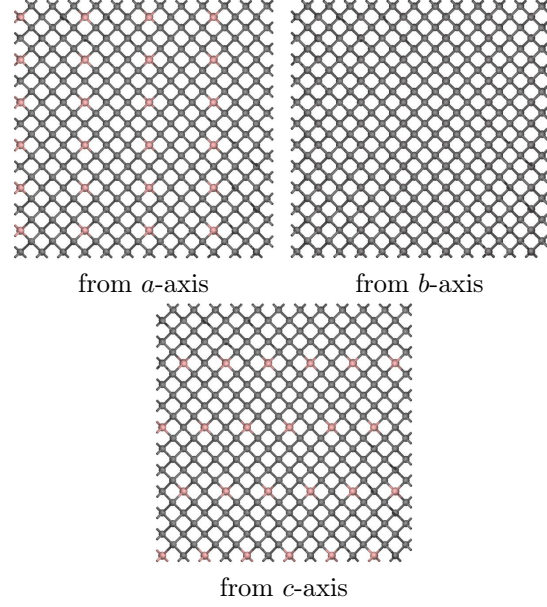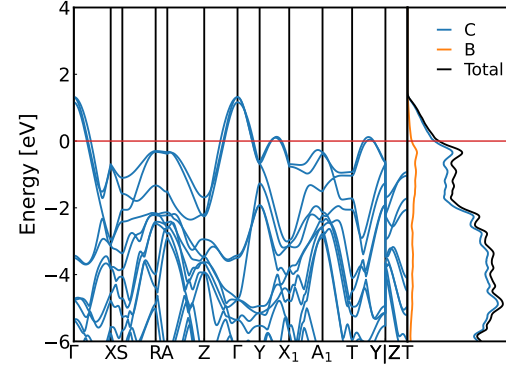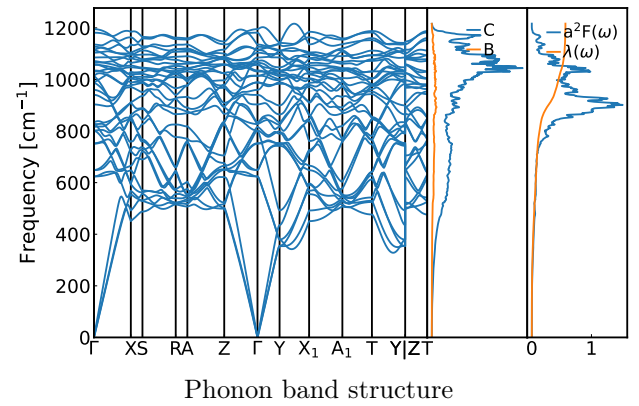

#4: B<sub>2</sub>C<sub>8</sub>Cl

mat id agm029547244  
 spg 225  
 nsites 11  
 e above hull 0.989 eV  
 e form 0.798 eV  
 decomposition B<sub>4</sub>C, BCl<sub>3</sub>, C  
 ecutwfc 90.0 Ry  
 kpts coarse 12×12×12  
 kpts fine 24×24×24  
 qpts 3×3×3  
 λ 3.278  
 ω<sub>log</sub> 294 K  
 ω<sub>2</sub> 492 K  
 T<sub>c</sub><sup>Mcmillan</sup> 55.0 K  
 T<sub>c</sub><sup>Allen-Dynes</sup> 82.7 K  
 T<sub>c</sub><sup>Eliashberg</sup> 96.1 K

**Primitive structure:**

$a$ : 4.9498 Å,  $b$ : 4.9498 Å,  $c$ : 4.9498 Å  
 $\alpha$ : 60.00°,  $\beta$ : 60.00°,  $\gamma$ : 60.00°

B [0.2500, 0.2500, 0.2500]  
 B [0.7500, 0.7500, 0.7500]  
 C [0.8879, 0.3364, 0.8879]  
 C [0.1121, 0.6636, 0.1121]  
 C [0.8879, 0.8879, 0.8879]  
 C [0.1121, 0.1121, 0.1121]  
 C [0.3364, 0.8879, 0.8879]  
 C [0.6636, 0.1121, 0.1121]  
 C [0.8879, 0.8879, 0.3364]  
 C [0.1121, 0.1121, 0.6636]  
 Cl [0.5000, 0.5000, 0.5000]

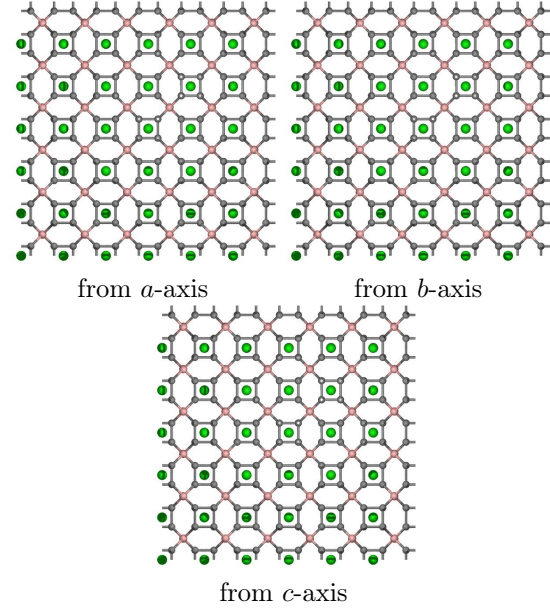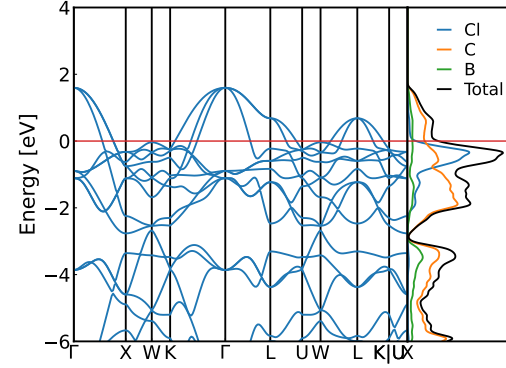

Electron band structure

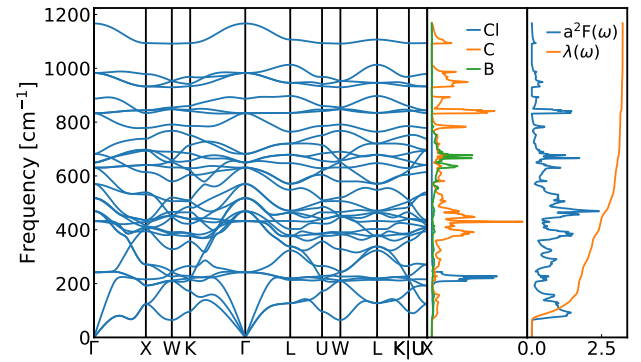

Phonon band structure

#5: Al<sub>2</sub>H<sub>7</sub>Os

mat id agm006206343  
 spg 225  
 nsites 10  
 e above hull 0.265 eV  
 e form 0.097 eV  
 decomposition Al<sub>2</sub>Os, H<sub>2</sub>  
 ecutwfc 86.0 Ry  
 kpts coarse 12×12×12  
 kpts fine 24×24×24  
 qpts 3×3×3  
 λ 3.175  
 ω<sub>log</sub> 204 K  
 ω<sub>2</sub> 596 K  
 T<sub>c</sub><sup>Mcmillan</sup> 37.6 K  
 T<sub>c</sub><sup>Allen-Dynes</sup> 57.3 K  
 T<sub>c</sub><sup>Eliashberg</sup> 100.0 K

**Primitive structure:**

$a$ : 4.5896 Å,  $b$ : 4.5896 Å,  $c$ : 4.5896 Å  
 $\alpha$ : 60.00°,  $\beta$ : 60.00°,  $\gamma$ : 60.00°

|    |                          |
|----|--------------------------|
| Al | [0.7500, 0.7500, 0.7500] |
| Al | [0.2500, 0.2500, 0.2500] |
| H  | [0.5000, 0.5000, 0.5000] |
| H  | [0.2721, 0.2721, 0.7279] |
| H  | [0.2721, 0.7279, 0.2721] |
| H  | [0.7279, 0.2721, 0.7279] |
| H  | [0.2721, 0.7279, 0.7279] |
| H  | [0.7279, 0.2721, 0.2721] |
| H  | [0.7279, 0.7279, 0.2721] |
| Os | [0.0000, 0.0000, 0.0000] |

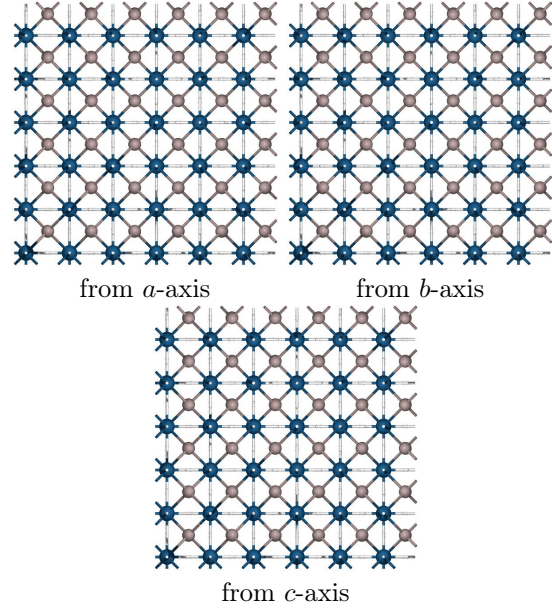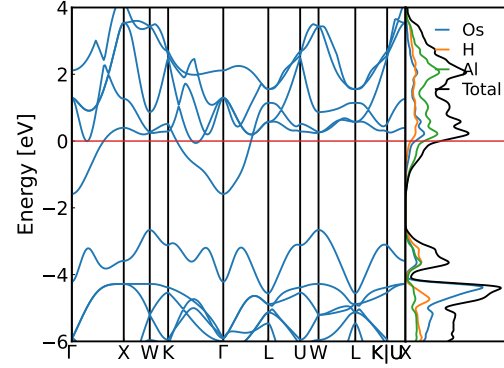

Electron band structure

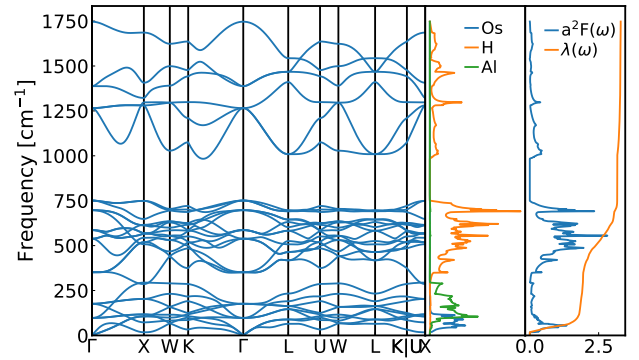

Phonon band structure

## #6: $\text{Li}_2\text{AgH}_6$

mat id agm006188332  
 spg 225  
 nsites 9  
 e above hull 0.319 eV  
 e form 0.094 eV  
 decomposition  $\text{LiH}_9$ , Ag, LiH  
 ecutwfc 104.0 Ry  
 kpts coarse  $12 \times 12 \times 12$   
 kpts fine  $24 \times 24 \times 24$   
 qpts  $3 \times 3 \times 3$   
 $\lambda$  3.783  
 $\omega_{\text{log}}$  338 K  
 $\omega_2$  655 K  
 $T_c^{\text{McMillan}}$  66.5 K  
 $T_c^{\text{Allen-Dynes}}$  110.6 K  
 $T_c^{\text{Eliashberg}}$  132.3 K

### Primitive structure:

$a$ : 4.6213 Å,  $b$ : 4.6213 Å,  $c$ : 4.6213 Å  
 $\alpha$ : 60.00°,  $\beta$ : 60.00°,  $\gamma$ : 60.00°

|    |                          |
|----|--------------------------|
| Li | [0.7500, 0.7500, 0.7500] |
| Li | [0.2500, 0.2500, 0.2500] |
| Ag | [0.0000, 0.0000, 0.0000] |
| H  | [0.2654, 0.2654, 0.7346] |
| H  | [0.2654, 0.7346, 0.2654] |
| H  | [0.7346, 0.2654, 0.7346] |
| H  | [0.7346, 0.7346, 0.2654] |
| H  | [0.2654, 0.7346, 0.7346] |
| H  | [0.7346, 0.2654, 0.2654] |

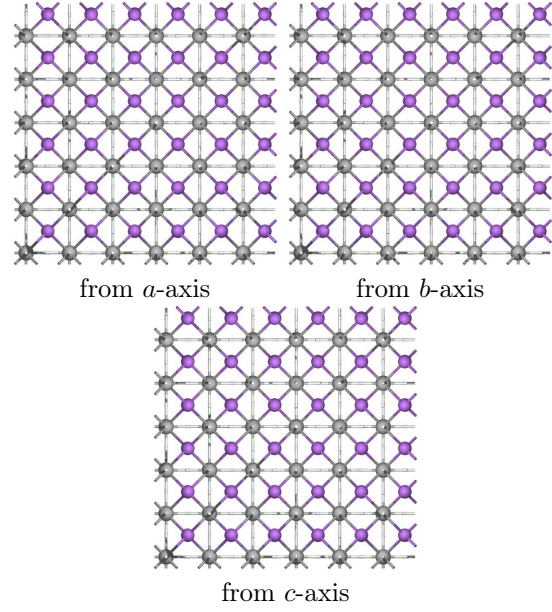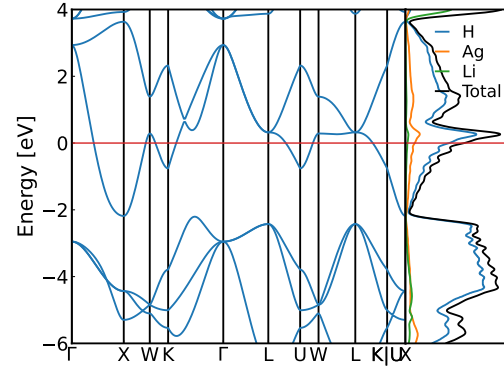

Electron band structure

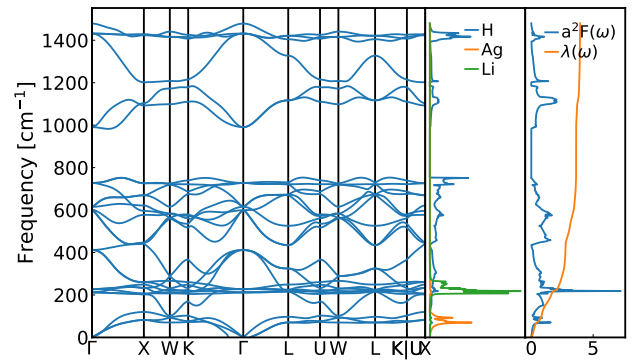

Phonon band structure

To address the anharmonic phonon properties of  $\text{Li}_2\text{AgH}_6$  and  $\text{Li}_2\text{AuH}_6$  at ambient pressure, we used the stochastic self-consistent harmonic approximation (SSCHA) method [1–4]. In the case of  $\text{Li}_2\text{AgH}_6$ , a  $4 \times 4 \times 4$  supercell including 576 atoms was used in SSCHA calculations, which corresponds to the dynamical matrices on a commensurate  $4 \times 4 \times 4$   $\mathbf{q}$ -mesh. All the degrees of freedom were fully relaxed in the SSCHA calculations. Due to the heavy DFT calculations and the demanding number of structure configurations used for the convergence of Hessian phonons, we trained a Gaussian approximation potential [5] based on the DFT calculations. The converged free energy Hessian phonons were obtained by using the Gaussian approximation potential. In the anharmonic phonon calculations of  $\text{Li}_2\text{AuH}_6$ , we employed  $2 \times 2 \times 2$  supercell with 72 atoms that is sufficient to get convergence. The cutoff energy was 80 Ry with  $10 \times 10 \times 10$   $\mathbf{k}$ -point grid for the supercell calculations. We also performed electron-phonon coupling calculations for the anharmonic structure of  $\text{Li}_2\text{AuH}_6$ , on  $6 \times 6 \times 6$   $\mathbf{q}$ -point grid with coarse  $\mathbf{k}$ -point sampling of  $24 \times 24 \times 24$  and dense grid of  $42 \times 42 \times 42$ . The double delta sum was done with 0.004 Ry Gaussian smearing. The results are summarized in Table S1.

TABLE S1. Calculated electron-phonon coupling constant,  $\omega_{\log}$ ,  $\omega_2$ , and  $T_c$  for  $\text{Li}_2\text{AuH}_6$ . The superconducting critical temperature is calculated with McMillan’s formula and Allen-Dynes modified formula (AD) with  $\mu^* = 0.1$ , with harmonic phonons and anharmonic phonons from the SSCHA auxiliary force constants and those from the SSCHA free energy Hessian.

| $\mu^* = 0.1$              | Harmonic | Auxiliary | Hessian |
|----------------------------|----------|-----------|---------|
| $\lambda$                  | 3.86     | 2.10      | 2.67    |
| $\omega_{\log}$ (K)        | 317      | 572       | 503     |
| $\omega_2$ (K)             | 724      | 982       | 870     |
| $T_c(\text{K})$ - McMillan | 63       | 85        | 86      |
| $T_c(\text{K})$ - AD       | 108      | 107       | 118     |

Fig. S1 shows the comparison between the harmonic phonons from DFPT, anharmonic free energy Hessian phonon spectra, and the anharmonic auxiliary phonon spectra for both  $\text{Li}_2\text{AgH}_6$  and  $\text{Li}_2\text{AuH}_6$ .

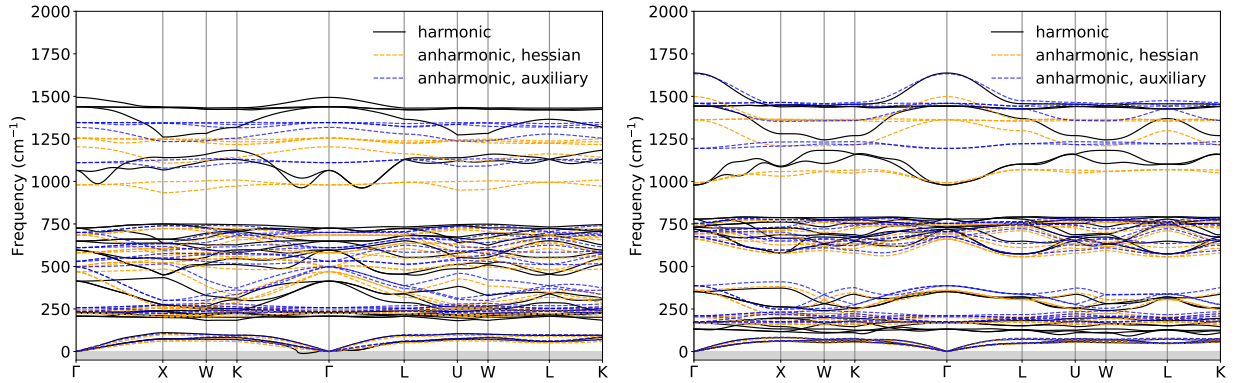

FIG. S1. Anharmonic free energy Hessian phonon spectra and anharmonic auxiliary phonon spectra of  $\text{Li}_2\text{AgH}_6$  (left panel) and  $\text{Li}_2\text{AuH}_6$  (right panel) calculated by the stochastic self-consistent harmonic approximation (SSCHA) at ambient pressure (the reader is referred to Refs. [2, 4] for details). The results are compared to the harmonic result. In the case of  $\text{Li}_2\text{AgH}_6$  anharmonicity lifts the instability observed close to  $\Gamma$  in the harmonic case.

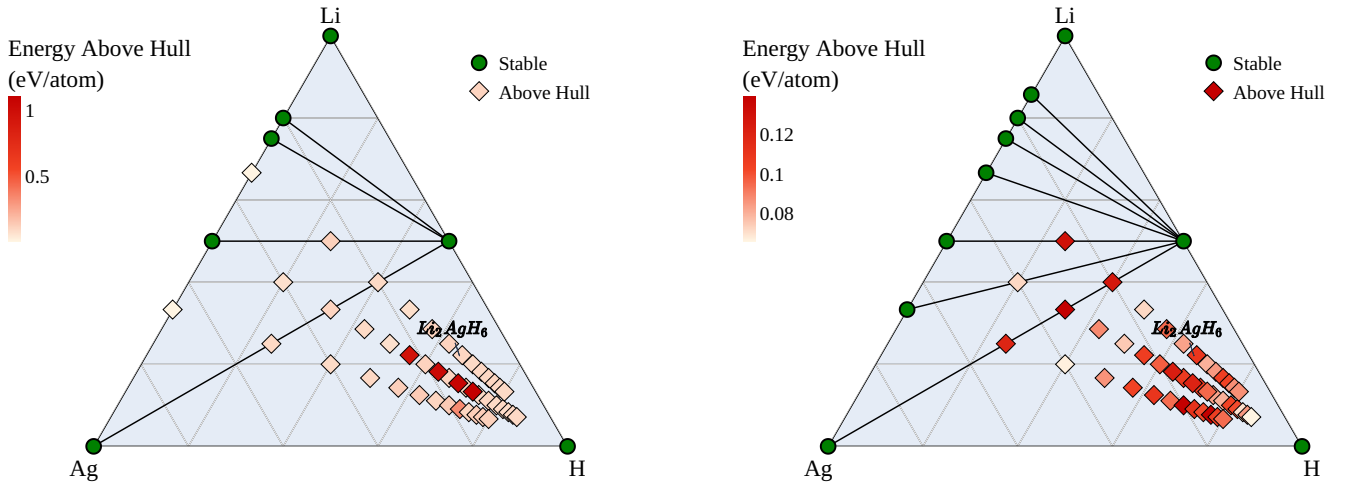

FIG. S2. The convex hull of the Li-Ag-H system at 25 GPa (left) and 50 GPa (right). Circles represent thermodynamically stable structures, and diamonds represent metastable structures.

- 
- [1] Errea, I., Calandra, M. & Mauri, F. Anharmonic free energies and phonon dispersions from the stochastic self-consistent harmonic approximation: Application to platinum and palladium hydrides. *Phys. Rev. B* **89**, 064302 (2014). URL <https://link.aps.org/doi/10.1103/PhysRevB.89.064302>.
  - [2] Bianco, R., Errea, I., Paulatto, L., Calandra, M. & Mauri, F. Second-order structural phase transitions, free energy curvature, and temperature-dependent anharmonic phonons in the self-consistent harmonic approximation: Theory and stochastic implementation. *Phys. Rev. B* **96**, 014111 (2017). URL <https://link.aps.org/doi/10.1103/PhysRevB.96.014111>.
  - [3] Monacelli, L., Errea, I., Calandra, M. & Mauri, F. Pressure and stress tensor of complex anharmonic crystals within the stochastic self-consistent harmonic approximation. *Phys. Rev. B* **98**, 024106 (2018). URL <https://link.aps.org/doi/10.1103/PhysRevB.98.024106>.
  - [4] Monacelli, L. *et al.* The stochastic self-consistent harmonic approximation: calculating vibrational properties of materials with full quantum and anharmonic effects. *J. Phys. Condens. Matter*. **33**, 363001 (2021). URL <https://doi.org/10.1088/1361-648x/ac066b>.
  - [5] Bartók, A. P., Payne, M. C., Kondor, R. & Csányi, G. Gaussian approximation potentials: The accuracy of quantum mechanics, without the electrons. *Phys. Rev. Lett.* **104**, 136403 (2010). URL <https://link.aps.org/doi/10.1103/PhysRevLett.104.136403>.
